# Supplementary material for: Flux-conserving diagrammatic formulation of optical spectroscopy of open quantum systems
Source: arXiv:1909.04829 source file (2019-09-11)
Supplement: Supplementary file 1 [file spectroscopy_si_v8.pdf]

# Supporting Information: Flux-conserving diagrammatic formulation of optical spectroscopy of open quantum systems

Shaul Mukamel*,† and Michael Galperin*,‡

†*Department of Chemistry, University of California Irvine, Irvine, CA 92697, USA*

‡*Department of Chemistry and Biochemistry, University of California San Diego, La Jolla, CA 92093, USA*

E-mail: smukamel@uci.edu; migalperin@ucsd.edu

Phone: +1 949 824 7600; +1 858 246 0511

# Expressions for NEGF self-energies

Expressions for the NEGF self-energies of electron due to coupling to photons $\Sigma^{pt}$, eq 22, and of photon due to coupling to electron sub-system $\Pi^{el}$, eq 23, are

$$
\begin{aligned}
&\Sigma^{pt}_{m_1m_2}(\tau_1,\tau_2) = \qquad\qquad\qquad\qquad\qquad\qquad\qquad\qquad\qquad\qquad\qquad\qquad\qquad\qquad \text{(S1)}\\
&i\sum_{\alpha_1,\alpha_2}\sum_{n_1,n_2\in M} G_{n_1n_2}(\tau_1,\tau_2)\Big(U_{n_1m_1,\alpha_1}F_{\alpha_1,\alpha_2}(\tau_1,\tau_2)U_{\alpha_2,n_2m_2} + U_{m_2n_2,\alpha_2}F_{\alpha_2\alpha_1}(\tau_2,\tau_1)U_{\alpha_1,m_1n_1}\Big)\\
&-\sum_{\substack{\alpha_1,\alpha_2\\ \alpha_3,\alpha_4}}\sum_{\substack{n_1,n_2,n_3\\ n_4,n_5,n_6\in M}}\int_c d\tau_3\int_c d\tau_4\, G_{n_1n_2}(\tau_1,\tau_3)\,G_{n_3n_4}(\tau_3,\tau_4)\,G_{n_5n_6}(\tau_4,\tau_2)\\
&\qquad\times\Big(U_{n_1m_1,\alpha_1}F_{\alpha_1\alpha_4}(\tau_1,\tau_4)U_{\alpha_4,n_4n_5} + U_{n_5n_4,\alpha_4}F_{\alpha_4\alpha_1}(\tau_4,\tau_1)U_{\alpha_1,m_1n_1}\Big)\\
&\qquad\times\Big(U_{m_2n_6,\alpha_2}F_{\alpha_2\alpha_3}(\tau_2,\tau_3)U_{\alpha_3,n_2n_3} + U_{n_3n_2,\alpha_3}F_{\alpha_3\alpha_2}(\tau_3,\tau_2)U_{\alpha_2,n_6m_2}\Big)\\
&\Pi^{el}_{\alpha_1\alpha_2}(\tau_1,\tau_2) = \qquad\qquad\qquad\qquad\qquad\qquad\qquad\qquad\qquad\qquad\qquad\qquad\qquad\qquad \text{(S2)}\\
&-i\sum_{\substack{n_1,n_2\\ n_3,n_4\in M}} U_{\alpha_1,n_1n_2}\,G_{n_2n_4}(\tau_1,\tau_2)\,G_{n_3n_1}(\tau_2,\tau_1)\,U_{n_3n_4,\alpha_2}\\
&+\sum_{\alpha_3,\alpha_4}\sum_{\substack{n_1,n_2,n_3,n_4\\ n_5,n_6,n_7,n_8\in M}}\int_c d\tau_3\int_c d\tau_4\, U_{\alpha_1,n_1n_2}U_{n_3n_4,\alpha_3}F_{\alpha_3\alpha_4}(\tau_3,\tau_4)U_{\alpha_4,n_7n_8}U_{n_5n_6,\alpha_2}\\
&\qquad\times\Big(G_{n_2n_4}(\tau_1,\tau_3)\,G_{n_3n_6}(\tau_3,\tau_2)\,G_{n_5n_7}(\tau_2,\tau_4)\,G_{n_8n_1}(\tau_4,\tau_1)\\
&\qquad\quad + G_{n_2n_7}(\tau_1,\tau_4)\,G_{n_8n_5}(\tau_4,\tau_2)\,G_{n_5n_4}(\tau_2,\tau_3)\,G_{n_3n_1}(\tau_3,\tau_1)\Big)
\end{aligned}
$$

Here first (second) term in the right-hand-side of the expressions represents second (fourth) order contribution to the self-energies.
